# Supplementary material for: Structural Patterns and Generative Models of Real-world Hypergraphs
Source: arXiv:2006.07060 source file (2020-06-12)
Supplement: Supplementary file 1 [file 071appendixB.tex]

\section{Appendix: Results of Generators}
\label{appendix:summary}

We present the patterns reproduced by each generator for the other 3 datasets mentioned in Table \ref{tab:counts}. In Table \ref{tab:summary_DAWN_Eu_tag-math}, in each decomposition level, each of the following entry is marked with \cmark if and only if:
\bit
\item{\bf P1. Giant Conn. Comp.}: the decomposed graph at that level of the generated hypergraph retains a giant connected component. If this entry is marked with \xmark, the entries of P3. and P4. at the same decomposition level will automatically be marked with \xmark, as explained in Section 4.1 and Section 4.3.
\item{\bf  P2. Heavy-tail Degree Dist.}: the decomposed graph at that level of the generated hypergraph possesses a degree distribution looking similar and having the highest degrees not too different from that of the original hypergraph.
\item{\bf P3. Small Diameter}: the decomposed graph at that level of the generated hypergraph has the effective diameter within a small deviation of the effective diameter $d$ of the original dataset. We adopt a heuristic of the acceptance range as $(\frac{2d}{3}, \frac{4d}{3})$.
\item{\bf P4. High Clustering Coeff.}: the decomposed graph at that level of the generated hypergraph has a clustering coefficient within a small deviation of the clustering coefficient $c$ of the original dataset. We adopt a heuristic of the acceptance range as $(\frac{2c}{3}, \max(\frac{4c}{3}, 1))$.
\item{\bf P5. Skewed Singular Val.}: the decomposed graph at that level has a skewed plot of singular values in the log-log scale.
\eit
